# Supplementary material for: Performance guarantees for model-based Approximate Dynamic Programming in continuous spaces
Source: arXiv:1602.07273 source file (2018-08-30)
Supplement: Supplementary file 1 [file 11_appendix_A_1norm_fitting.tex]

% !TEX root = ../root.tex
%%%%%%%%%%%%%%%%%%%%%%%%%%%%%%%%%%%%%%%%%%%%%%%%%%%%%%%%%%%%%%%%%%%%%%%%%%%%%%%%
%2345678901234567890123456789012345678901234567890123456789012345678901234567890
%        1         2         3         4         5         6         7         8

%\section{Appendix A: Proofs} \label{app:proofs}
%\section{test}
%\subsection{test2}

\subsection{Proofs of equivalence with 1-norm fitting} \label{app:1norm_equivalence}

\itshape Lemma \ref{lemma:approxLP_for_Q_solves_min_1norm}: \normalfont
	An approximate $\mcal{Q}$-function, $\hat{Q}$, solves \eqref{eq:LP_approach_to_ADP_iterated_Qform}, if and only if it solves a minimisation optimisation problem with the same decision variables, same constraints, and the objective replaced by,
	\begin{equation} \nonumber
		\begin{aligned}
			\left\| \, Q^\ast \,-\, \hat{Q} \, \right\|_{1,c(x,u)}
		\end{aligned}
	\end{equation}
%\end{lemma}

\vspace{0.2cm}

\begin{proof}
	As the operator $F$ is monotonic and contractive (see Proposition \ref{proposition:operator_properties}), with fixed point $Q^\ast(x)$, the constraints of \eqref{eq:LP_approach_to_ADP_iterated_Qform} enforce that any feasible $\hat{Q}$ satisfies $\hat{Q}(x,u) \,\leq\,  Q^\ast(x,u)$ for all $\xinX$ and $\uinU$. Thus the objective of the 1-norm minimisation can be written out as,
	\begin{equation} \nonumber
		\begin{aligned}
			&\, \left\|\, Q^\ast - \hat{Q} \,\right\|_{1,c(x,u)}
			\\
			=&\, \int\nolimits_{\mcal{X}} \, c(x,u) \, \left|\, Q^\ast(x,u) - \hat{Q}(x,u) \,\right|
			\\
			%=&\, \int_{\mcal{X}} \, c(x) \, \left(\, V^\ast(x) - \hat{V}(x) \,\right)
			%\\
			=&\, \underbrace{\left( \int\nolimits_{\mcal{X}\times\mcal{U}} \, c(x,u) \, Q^\ast(x,u) \right)}_{\text{a constant}} \,-\, \left( \int\nolimits_{\mcal{X}\times\mcal{U}} c(x,u) \, \hat{Q}(x,u) \,\right)
		\end{aligned}
	\end{equation}
	
	The first term in the last equivalence is a constant relative to the optimisation variable $\hat{Q}$. Therefore, maximising $\int\nolimits_{\mcal{X}\times\mcal{U}} \, c(x,u) \hat{Q}(x,u)$ is equivalent to minimising of the 1-norm of the difference. As both optimisation problems have the same decision variables and constraints, the problems are equivalent.
	%
	%The Bellman operator, $\mcal{T}$, is also monotone and contractive, hence the same argument holds for the value function formulation.
\end{proof}

\vspace{0.2cm}

Note that this proof will hold for any constraint that implies $\hat{Q} \leq Q^\ast$, as long as the two optimisation programs have the same constraint.
